# Supplementary material for: DualNeRF: Text-Driven 3D Scene Editing via Dual-Field Representation
Source: arXiv:2502.16302 source file (2025-02-22)
Supplement: Supplementary file 1 [file X_suppl.tex]

\clearpage
\setcounter{page}{1}
\maketitlesupplementary

\section{Additional Implementation Details}
\label{sec: Additional Implementation Details}
For the static field $f_S$ in DualNeRF, we first train it for $30k$ iterations per scene based on the \textit{nerfacto} model in NeRFStudio \cite{nerfstudio} following \cite{haque2023instruct}. This process takes about $15$ minutes on a single NVIDIA GeForce RTX 3090. The dynamic field is then trained for $15k$ iterations to perform editing, which takes about one hour on a single NVIDIA GeForce RTX 3090. Each round of IDU contains a dataset updating step with $d = 1$ and a NeRF updating step with $ n = 10$. In other words, we alternatively update one image in the training dataset and train DualNeRF for $10$ iterations, following \cite{haque2023instruct}. The classifier-free guidance weight of InstructPix2pix \cite{brooks2023instructpix2pix} is fixed at $s_I = 1.5$, $s_T = 7.5$ for each scene. We do not make any adjustment to these two weights as IN2N \cite{haque2023instruct} since this behavior is irrelevant to our work. All the other training parameters follow the default setting of NeRFStudio \cite{nerfstudio}. For IP2P \cite{brooks2023instructpix2pix} and CLIP model \cite{radford2021learning}, we use the implementation provided in website \textit{https://huggingface.co/}.

\section{Metrics}
\label{sec: Metrics}
As we mentioned in \ref{sec: Evaluation Criteria} and \ref{sec: Quantitative Results}, quantitative comparisons are conducted between DualNeRF and baselines across $3$ scenes over $10$ edits. Detailed information and experimental results of these $10$ edits are shown in Tab. \ref{tab: detailed results}. Metrics used in these experiments include SSIM \cite{wang2004image} and two CLIP-based metrics used in \cite{haque2023instruct}, namely the CLIP text-image direction similarity $C_{t2i}$ and CLIP direction consistency $C_{dir}$.

CLIP text-image direction similarity $C_{t2i}$ is calculated as the cosine similarity between the direction vector $\mathbf{v}_{img}$ from the CLIP embedding of the original image $\mathbf{e}_{img}^{(o)}$ to the edited image $\mathbf{e}_{img}^{(e)}$ and the direction vector $\mathbf{v}_{text}$ from the CLIP embedding of the original image's caption $\mathbf{e}_{text}^{(o)}$ to the edited caption $\mathbf{e}_{text}^{(e)}$:
\begin{equation}
    C_{t2i} = \frac{\mathbf{v}_{img} \cdot \mathbf{v}_{text}}{||\mathbf{v}_{img}||_2||\mathbf{v}_{text}||_2}
\end{equation}
where 
\begin{equation}
    \mathbf{v}_{img} = \mathbf{e}_{img}^{(e)} - \mathbf{e}_{img}^{(o)}
\end{equation}
\begin{equation}
    \mathbf{v}_{text} = \mathbf{e}_{text}^{(e)} - \mathbf{e}_{text}^{(o)}
\end{equation}
The captions of the original image and edited image comply with the format of ``A photograph of a $<$item$>$", where ``$<$item$>$" is a specific noun (phrase) describing the corresponding target in the image, following \cite{haque2023instruct}. For example, for the scene $person$ with the prompt ``As a bronze statue", the captions of the original image and edited image are set as ``A photograph of a person" and ``A photograph of a bronze statue" respectively.

CLIP direction consistency $C_{dir}$ is calculated as the average value among cosine similarities between several pairs of rendering results of the edited model with two close enough camera poses, following \cite{haque2023instruct}. More concretely, given a pair of camera poses $P_1$ and $P_2$ which are close enough to each other (we abuse the subscript here), we render the model under these two camera poses, generating two renderings $I_1$ and $I_2$. The CLIP direction consistency between these two renderings is defined as the inner product of the normalized CLIP embeddings of these two images:
\begin{equation}
    C_{dir}(I_1, I_2) = \frac{E_{I}(I_1) \cdot E_{I}(I_2)}{||E_{I}(I_1)||_2||E_{I}(I_2)||_2}
\end{equation}
where $E_{I}$ is the image encoder of CLIP as mentioned in Sec. \ref{sec: Editing Result Filtering}. The final CLIP direction consistency $C_{dir}$ of an edit is calculated as the average value of several sampling pairs of adjacent renderings.
% \begin{equation}
%     C_{dir} = \frac{1}{|\mathcal{I}_{dir}|}\sum_{(I_1, I_2) \in \mathcal{I}_{dir}}C_{t2i}(I_1, I_2)
% \end{equation}
% where $\mathcal{I}_{dir}$ is the set of sampling pairs.

\section{Detailed Architecture of DualNeRF}
We also display the detailed architecture of DualNeRF in Fig. \ref{fig: detailed architecture}. As we can see from Fig. \ref{fig: detailed architecture}, each field in DualNeRF mainly contains two modules: a density module that is only conditioned on $\mathbf{x}$, and a color module that is conditioned on both $\mathbf{d}$ and a hidden feature $\mathbf{h}$ generated by the density module, following the design of \cite{mildenhall2021nerf}.

\begin{figure}[t]
    \centering
    \includegraphics[width=1.0\linewidth]{fig/supply_architecture.pdf}
    \caption{\textbf{Detailed Architecture of DualNeRF.} The detailed architecture of DualNeRF is shown in this image. $\mathbf{h}^{(S)}$ and $\mathbf{h}^{(D)}$ are two hidden features transferred between the density module and color module.}
    \label{fig: detailed architecture}
\end{figure}

\section{More Qualitative Results}
\label{sec: More Qualitative Results}
More qualitative results of DualNeRF are displayed in Fig. \ref{fig: more qualitative results}. We show results across different scenes with diverse prompts ranging from ``Turn the bear into a grizzly bear" to ``Turn him into Michael Jackson". As we can see from Fig. \ref{fig: more qualitative results}, our model generates brilliant results under various settings, which demonstrates the effectiveness and versatility of DualNeRF.

\begin{figure*}[htbp]
    \centering

    \begin{subfigure}{0.19\linewidth}
        \begin{minipage}[t]{1.0\linewidth}
            \centering
            \includegraphics[width=1.0\linewidth]{fig/bear1.pdf}
            % \caption{Original Scene}
        \end{minipage}
    \end{subfigure}
    \hfill
    \begin{subfigure}{0.19\linewidth}
        \begin{minipage}[t]{1.0\linewidth}
            \centering
            \includegraphics[width=1.0\linewidth]{fig/bear2.pdf}
            % \caption{w/o SA and CCI}
        \end{minipage}
    \end{subfigure}
    \hfill
    \begin{subfigure}{0.19\linewidth}
        \begin{minipage}[t]{1.0\linewidth}
            \centering
            \includegraphics[width=1.0\linewidth]{fig/bear3.pdf}
            % \caption{w/o CCI}
        \end{minipage}
    \end{subfigure}
    \hfill
    \begin{subfigure}{0.19\linewidth}
        \begin{minipage}[t]{1.0\linewidth}
            \centering
            \includegraphics[width=1.0\linewidth]{fig/bear4.pdf}
            % \caption{w/o CCI}
        \end{minipage}
    \end{subfigure}
    \hfill
    \begin{subfigure}{0.19\linewidth}
        \begin{minipage}[t]{1.0\linewidth}
            \centering
            \includegraphics[width=1.0\linewidth]{fig/bear5.pdf}
            % \caption{w/o CCI}
        \end{minipage}
    \end{subfigure}

    \begin{subfigure}{0.19\linewidth}
        \begin{minipage}[t]{1.0\linewidth}
            \centering
            \includegraphics[width=1.0\linewidth]{fig/face1.pdf}
            % \caption{Original Scene}
        \end{minipage}
    \end{subfigure}
    \hfill
    \begin{subfigure}{0.19\linewidth}
        \begin{minipage}[t]{1.0\linewidth}
            \centering
            \includegraphics[width=1.0\linewidth]{fig/face2.pdf}
            % \caption{w/o SA and CCI}
        \end{minipage}
    \end{subfigure}
    \hfill
    \begin{subfigure}{0.19\linewidth}
        \begin{minipage}[t]{1.0\linewidth}
            \centering
            \includegraphics[width=1.0\linewidth]{fig/face3.pdf}
            % \caption{w/o CCI}
        \end{minipage}
    \end{subfigure}
    \hfill
    \begin{subfigure}{0.19\linewidth}
        \begin{minipage}[t]{1.0\linewidth}
            \centering
            \includegraphics[width=1.0\linewidth]{fig/face4.pdf}
            % \caption{w/o CCI}
        \end{minipage}
    \end{subfigure}
    \hfill
    \begin{subfigure}{0.19\linewidth}
        \begin{minipage}[t]{1.0\linewidth}
            \centering
            \includegraphics[width=1.0\linewidth]{fig/face5.pdf}
            % \caption{w/o CCI}
        \end{minipage}
    \end{subfigure}

    \begin{subfigure}{0.19\linewidth}
        \begin{minipage}[t]{1.0\linewidth}
            \centering
            \includegraphics[width=1.0\linewidth]{fig/person1.pdf}
            % \caption{Original Scene}
        \end{minipage}
    \end{subfigure}
    \hfill
    \begin{subfigure}{0.19\linewidth}
        \begin{minipage}[t]{1.0\linewidth}
            \centering
            \includegraphics[width=1.0\linewidth]{fig/person2.pdf}
            % \caption{w/o SA and CCI}
        \end{minipage}
    \end{subfigure}
    \hfill
    \begin{subfigure}{0.19\linewidth}
        \begin{minipage}[t]{1.0\linewidth}
            \centering
            \includegraphics[width=1.0\linewidth]{fig/person3.pdf}
            % \caption{w/o CCI}
        \end{minipage}
    \end{subfigure}
    \hfill
    \begin{subfigure}{0.19\linewidth}
        \begin{minipage}[t]{1.0\linewidth}
            \centering
            \includegraphics[width=1.0\linewidth]{fig/person4.pdf}
            % \caption{w/o CCI}
        \end{minipage}
    \end{subfigure}
    \hfill
    \begin{subfigure}{0.19\linewidth}
        \begin{minipage}[t]{1.0\linewidth}
            \centering
            \includegraphics[width=1.0\linewidth]{fig/person5.pdf}
            % \caption{w/o CCI}
        \end{minipage}
    \end{subfigure}

    \begin{subfigure}{0.19\linewidth}
        \begin{minipage}[t]{1.0\linewidth}
            \centering
            \includegraphics[width=1.0\linewidth]{fig/fangzhou1.pdf}
            % \caption{Original Scene}
        \end{minipage}
    \end{subfigure}
    \hfill
    \begin{subfigure}{0.19\linewidth}
        \begin{minipage}[t]{1.0\linewidth}
            \centering
            \includegraphics[width=1.0\linewidth]{fig/fangzhou2.pdf}
            % \caption{w/o SA and CCI}
        \end{minipage}
    \end{subfigure}
    \hfill
    \begin{subfigure}{0.19\linewidth}
        \begin{minipage}[t]{1.0\linewidth}
            \centering
            \includegraphics[width=1.0\linewidth]{fig/fangzhou3.pdf}
            % \caption{w/o CCI}
        \end{minipage}
    \end{subfigure}
    \hfill
    \begin{subfigure}{0.19\linewidth}
        \begin{minipage}[t]{1.0\linewidth}
            \centering
            \includegraphics[width=1.0\linewidth]{fig/fangzhou4.pdf}
            % \caption{w/o CCI}
        \end{minipage}
    \end{subfigure}
    \hfill
    \begin{subfigure}{0.19\linewidth}
        \begin{minipage}[t]{1.0\linewidth}
            \centering
            \includegraphics[width=1.0\linewidth]{fig/fangzhou5.pdf}
            % \caption{w/o CCI}
        \end{minipage}
    \end{subfigure}
    
    \caption{\textbf{More Qualitative Results.} More quantitative results of DualNeRF are shown in this figure, demonstrating the effectiveness and versatility of DualNeRF.}
    \label{fig: more qualitative results}
\end{figure*}

\begin{table*}[htbp]
    \centering
    % \rowcolors{1}{white}{gray!20}
    \begin{tabular}{p{32pt}<{\centering}|p{145pt}<{\centering}|p{25pt}<{\centering}|p{25pt}<{\centering}|p{25pt}<{\centering}|p{25pt}<{\centering}|p{25pt}<{\centering}|p{25pt}<{\centering}|p{25pt}<{\centering}|p{25pt}<{\centering}|p{25pt}<{\centering}}
    \toprule
    \multirow{2}{*}{Scene} & \multirow{2}{*}{Prompt} & \multicolumn{3}{c|}{Per-frame IP2P} & \multicolumn{3}{c|}{IN2N} & \multicolumn{3}{c}{DualNeRF} \\
    \cline{3-11}
     &  & $C_{t2i}$ & $C_{dir}$ & $SSIM$ & $C_{t2i}$ & $C_{dir}$ & $SSIM$ & $C_{t2i}$ & $C_{dir}$ & $SSIM$ \\
    \midrule
    \multirow{5}{*}{\textit{person}} & As a bronze statue & $0.1883$ & $0.9588$ & $0.8071$ & $0.1850$ & $0.9798$ & $0.8076$ & $0.1875$ & $0.9809$ & $0.8082$ \\
     & Put him in a suit & $0.2456$ & $0.9488$ & $0.8692$ & $0.2260$ & $0.9780$ & $0.8572$ & $0.2173$ & $0.9752$ & $0.8588$ \\
     & Turn him into a clown & $0.2397$ & $0.9559$ & $0.8832$ & $0.2539$ & $0.9812$ & $0.8621$ & $0.2537$ & $0.9752$ & $0.8721$ \\
     & Make him a marble statue & $0.1532$ & $0.9315$ & $0.8475$ & $0.1519$ & $0.9836$ & $0.8257$ & $0.1320$ & $0.9807$ & $0.8284$ \\
     & Turn him into a firefighter with a hat
     & $0.2638$ & $0.9206$ & $0.8448$ & $0.2763$ & $0.9783$ & $0.8152$ & $0.2856$ & $0.9766$ & $0.8385$ \\
    \hline
    \multirow{2}{*}{\textit{fangzhou}} & Turn him into the Tolkien Elf
 & $0.2225$ & $0.9756$ & $0.7896$ & $0.2023$ & $0.9918$ & $0.5273$ & $0.2185$ & $0.9890$ & $0.5835$ \\
     & Turn him into Lord Voldemort
 & $0.1554$ & $0.9442$ & $0.8214$ & $0.1675$ & $0.9896$ & $0.6424$ & $0.1376$ & $0.9870$ & $0.6455$ \\
    \hline
    \multirow{3}{*}{\textit{face}} & Turn him into a clown
 & $0.2433$ & $0.9636$ & $0.7574$ & $0.2378$ & $0.9836$ & $0.6388$ & $0.2537$ & $0.9796$ & $0.6423$ \\
     & Turn him into Albert Einstein
 & $0.2255$ & $0.9332$ & $0.7547$ & $0.2234$ & $0.9658$ & $0.6467$ & $0.2295$ & $0.9622$ & $0.6423$ \\
     & Turn his face into a skull
 & $0.2261$ & $0.9029$ & $0.7780$ & $0.2459$ & $0.9747$ & $0.6307$ & $0.2746$ & $0.9702$ & $0.6423$ \\
    \hline
    \multicolumn{2}{c|}{Average} & $0.2153$ & $0.9435$ & $\boldsymbol{0.8194}$ & $0.2170$ & $\boldsymbol{0.9806}$ & $0.7254$ & $\boldsymbol{0.2190}$ & $0.9777$ & $0.7362$ \\
    \bottomrule
    \end{tabular}
    \caption{\textbf{Detailed Quantitative Results.} Experiments are conducted between DualNeRF and baselines across three scenes, including \textit{person}, \textit{fangzhou}, and \textit{face}, over $10$ edits shown in this table. The metrics used includes $C_{t2i}$, $C_{dir}$, and $SSIM$.}
    \label{tab: detailed results}
\end{table*}
